# Supplementary material for: Assessing impacts of discrepancies in model parameters on autoignition model performance: a case study using butanol
Source: arXiv:1708.02232 ancillary file (2017-12-24)
Supplement: Supplementary file 1 [file supplement.pdf]

# Assessing impacts of discrepancies in model parameters on autoignition model performance: a case study using butanol

Sai Krishna Sirumalla[a], Morgan A. Mayer[b], Kyle E. Niemeyer[b], Richard H. West[a,*]

[a] *Department of Chemical Engineering*
*Northeastern University, Boston, MA 02115, USA*
[b] *School of Mechanical, Industrial, and Manufacturing Engineering*
*Oregon State University, Corvallis, OR 97331, USA*

---

**Supplementary Material**

The full list of models considered, in alphabetical order of short-hand name. These models are available in: R. H. West, Combustion mechanism importer and kinetic models, Figshare (2017). doi:10.6084/m9.figshare.4787893.v1.

---

*Corresponding author
*Email address:* r.west@northeastern.edu (Richard H. West)

**AramcoMech_1.3**

AramcoMech 1.3 is a newly developed detailed chemical kinetic mechanism that characterises the kinetic and thermochemical properties of a large number of C1-C4 based hydrocarbon and oxygenated fuels over a wide range of experimental conditions. It was developed by the Combustion Chemistry Centre in NUI Galway and fully funded by Saudi Aramco.

W. K. Metcalfe, S. M. Burke, S. S. Ahmed, H. J. Curran A Hierarchical and Comparative Kinetic Modeling Study of C1-C2 Hydrocarbon and Oxygenated Fuels Intl. J. Chemical Kinetics 45 (2013) 638-675.

Downloaded in September 2013 from
http://c3.nuigalway.ie/Mechanism_release/download.html

**AramcoMech_2.0**

AramcoMech2.0 builds upon AramcoMech1.3 and has been developed to characterise the kinetic and thermochemical properties of a large number of C1–C4 based hydrocarbon and oxygenated fuels over a wide range of experimental conditions. It was developed by the Combustion Chemistry Centre at NUI Galway and has been funded by Saudi Aramco.

http://www.nuigalway.ie/c3/aramco2/frontmatter.html

**AutoTST-OOHabstraction**

Reaction rates for hydrogen abstraction reactions by OOH radical calculated using the Automated TST algorithm described in "Automated Transition State Theory Calculations for High-Throughput Kinetics" Pierre L Bhoorasingh, Belinda L Slakman, Fariba Seyedzadeh Khanshan, Jason Y Cain, and Richard H West The Journal of Physical Chemistry A (2017)

https://doi.org/10.1021/acs.jpca.7b07361

Including the data in Bhoorasingh, Pierre; Slakman, Belinda; Khanshan, Fariba Seyedzadeh; Cain, Jason; West, Richard (2016): Kinetic data for manuscript describing the AutoTST algorithm for automated Transition State Theory calculations of chemical reaction rates. figshare.

https://doi.org/10.6084/m9.figshare.4234160.v1

**Biomass**

Ranzi's biomass pyrolysis model, added to our database in July 2013, presumably from http://creckmodeling.chem.polimi.it

**Chernov**

Chernov, Victor, et al. "Soot formation with C1 and C2 fuels using an improved chemical mechanism for PAH growth." Combustion and Flame 161.2 (2014): 592-601.

https://doi.org/10.1016/j.combustflame.2013.09.017

**CombFlame2012/2028-Sarathy**

S. Mani Sarathy, Stijn Vranckx, Kenji Yasunaga, Marco Mehl, Patrick

Oßwald, Wayne K. Metcalfe, Charles K. Westbrook, William J. Pitz, Katharina Kohse-Höinghaus, Ravi X. Fernandes, Henry J. Curran, A comprehensive chemical kinetic combustion model for the four butanol isomers, Combustion and Flame, Volume 159, Issue 6, June 2012, Pages 2028-2055,

https://doi.org/10.1016/j.combustflame.2011.12.017.

**CombFlame2013/1315-Chang**

Yachao Chang, Ming Jia, Yaodong Liu, Yaopeng Li, Maozhao Xie, Development of a new skeletal mechanism for n-decane oxidation under engine-relevant conditions based on a decoupling methodology, Combustion and Flame, Volume 160, Issue 8, August 2013, Pages 1315-1332,

https://doi.org/10.1016/j.combustflame.2013.02.017.

**CombFlame2013/1541-Zhang**

Jiaxiang Zhang, Lun Pan, Jun Mo, Jing Gong, Zuohua Huang, Chung K. Law, A shock tube and kinetic modeling study of n-butanal oxidation, Combustion and Flame, Volume 160, Issue 9, September 2013, Pages 1541-1549,

https://doi.org/10.1016/j.combustflame.2013.04.002.

**CombFlame2013/1609-Veloo**

Peter S. Veloo, Philippe Dagaut, Casimir Togbé, Guillaume Dayma, S. Mani Sarathy, Charles K. Westbrook, Fokion N. Egolfopoulos, Experimental and modeling study of the oxidation of n- and iso-butanal, Combustion and Flame, Volume 160, Issue 9, September 2013, Pages 1609-1626,

https://doi.org/10.1016/j.combustflame.2013.03.018.

**CombFlame2013/17-Malewicki**

Tomasz Malewicki, Soumya Gudiyella, Kenneth Brezinsky, Experimental and modeling study on the oxidation of Jet A and the n-dodecane/iso-octane/n-propylbenzene/1,3,5-trimethylbenzene surrogate fuel, Combustion and Flame, Volume 160, Issue 1, January 2013, Pages 17-30,

https://doi.org/10.1016/j.combustflame.2012.09.013.

**CombFlame2013/1939-Cai**

Jianghuai Cai, Wenhao Yuan, Lili Ye, Zhanjun Cheng, Yizun Wang, Lidong Zhang, Feng Zhang, Yuyang Li, Fei Qi, Experimental and kinetic modeling study of 2-butanol pyrolysis and combustion, Combustion and Flame, Volume 160, Issue 10, October 2013, Pages 1939-1957,

https://doi.org/10.1016/j.combustflame.2013.04.010.

**CombFlame2013/1958-Zhao**

Long Zhao, Mingfeng Xie, Lili Ye, Zhanjun Cheng, Jianghuai Cai, Yuyang Li, Fei Qi, Lidong Zhang, An experimental and modeling study of methyl

propanoate pyrolysis at low pressure, Combustion and Flame, Volume 160, Issue 10, October 2013, Pages 1958-1966,

https://doi.org/10.1016/j.combustflame.2013.04.022.

**CombFlame2013/2291-Somers**

Kieran P. Somers, John M. Simmie, Fiona Gillespie, Christine Conroy, Gráinne Black, Wayne K. Metcalfe, Frédérique Battin-Leclerc, Patricia Dirrenberger, Olivier Herbinet, Pierre-Alexandre Glaude, Philippe Dagaut, Casimir Togbé, Kenji Yasunaga, Ravi X. Fernandes, Changyoul Lee, Rupali Tripathi, Henry J. Curran, A comprehensive experimental and detailed chemical kinetic modelling study of 2,5-dimethylfuran pyrolysis and oxidation, Combustion and Flame, Volume 160, Issue 11, November 2013, Pages 2291-2318,

https://doi.org/10.1016/j.combustflame.2013.06.007.

**CombFlame2013/2680-Vranckx**

Stijn Vranckx, Joachim Beeckmann, Wassja Alexander Kopp, Changyoul Lee, Liming Cai, Harish Kumar Chakravarty, Herbert Olivier, Kai Leonhard, Heinz Pitsch, Ravi Xavier Fernandes, An experimental and kinetic modelling study of n-butyl formate combustion, Combustion and Flame, Volume 160, Issue 12, December 2013, Pages 2680-2692,

https://doi.org/10.1016/j.combustflame.2013.06.012.

**CombFlame2013/2712-Sarathy**

S. Mani Sarathy, Sungwoo Park, Bryan W. Weber, Weijing Wang, Peter S. Veloo, Alexander C. Davis, Casimir Togbe, Charles K. Westbrook, Okjoo Park, Guillaume Dayma, Zhaoyu Luo, Matthew A. Oehlschlaeger, Fokion N. Egolfopoulos, Tianfeng Lu, William J. Pitz, Chih-Jen Sung, Philippe Dagaut, A comprehensive experimental and modeling study of iso-pentanol combustion, Combustion and Flame, Volume 160, Issue 12, December 2013, Pages 2712-2728,

https://doi.org/10.1016/j.combustflame.2013.06.022.

**CombFlame2013/487-Schenk**

Marina Schenk, Larisa Leon, Kai Moshammer, Patrick Oßwald, Thomas Zeuch, Lars Seidel, Fabian Mauss, Katharina Kohse-Höinghaus, Detailed mass spectrometric and modeling study of isomeric butene flames, Combustion and Flame, Volume 160, Issue 3, March 2013, Pages 487-503,

https://doi.org/10.1016/j.combustflame.2012.10.023.

**CombFlame2014/1135-Dames**

Enoch E. Dames, King-Yiu Lam, David F. Davidson, Ronald K. Hanson, An improved kinetic mechanism for 3-pentanone pyrolysis and oxidation developed using multispecies time histories in shock-tubes, Combustion and Flame, Volume 161, Issue 5, May 2014, Pages 1135-1145,

https://doi.org/10.1016/j.combustflame.2013.11.010.

**CombFlame2014/405-Cai**
Liming Cai, Heinz Pitsch, Mechanism optimization based on reaction rate rules, Combustion and Flame, Volume 161, Issue 2, February 2014, Pages 405-415,

https://doi.org/10.1016/j.combustflame.2013.08.024.

**CombFlame2014/65-Darcy**
D. Darcy, H. Nakamura, C.J. Tobin, M. Mehl, W.K. Metcalfe, W.J. Pitz, C.K. Westbrook, H.J. Curran, A high-pressure rapid compression machine study of n-propylbenzene ignition, Combustion and Flame, Volume 161, Issue 1, January 2014, Pages 65-74,

https://doi.org/10.1016/j.combustflame.2013.08.001.

**CombFlame2014/657-Jin**
Hanfeng Jin, Alberto Cuoci, Alessio Frassoldati, Tiziano Faravelli, Yizun Wang, Yuyang Li, Fei Qi, Experimental and kinetic modeling study of PAH formation in methane coflow diffusion flames doped with n-butanol, Combustion and Flame, Volume 161, Issue 3, March 2014, Pages 657-670,

https://doi.org/10.1016/j.combustflame.2013.10.020.

**CombFlame2014/798-Cai**
Liming Cai, Alena Sudholt, Dong Joon Lee, Fokion N. Egolfopoulos, Heinz Pitsch, Charles K. Westbrook, S. Mani Sarathy, Chemical kinetic study of a novel lignocellulosic biofuel: Di-n-butyl ether oxidation in a laminar flow reactor and flames, Combustion and Flame, Volume 161, Issue 3, 2014, Pages 798-809,

https://doi.org/10.1016/j.combustflame.2013.10.003.

**CombFlame2014/818-Zhang**
Kuiwen Zhang, Casimir Togbé, Guillaume Dayma, Philippe Dagaut, Experimental and kinetic modeling study of trans-methyl-3-hexenoate oxidation in JSR and the role of CC double bond, Combustion and Flame, Volume 161, Issue 3, March 2014, Pages 818-825,

https://doi.org/10.1016/j.combustflame.2013.10.022.

**CombFlame2014/84-Wang**
Zhandong Wang, Lili Ye, Wenhao Yuan, Lidong Zhang, Yizun Wang, Zhanjun Cheng, Feng Zhang, Fei Qi, Experimental and kinetic modeling study on methylcyclohexane pyrolysis and combustion, Combustion and Flame, Volume 161, Issue 1, January 2014, Pages 84-100,

https://doi.org/10.1016/j.combustflame.2013.08.011.

**CombFlame2014/885-Xiong**
Shao-Zhuan Xiong, Qian Yao, Ze-Rong Li, Xiang-Yuan Li, Reaction of ketenyl radical with hydroxyl radical over C2H2O2 potential energy surface: A theoretical study, Combustion and Flame, Volume 161, Issue 4, April 2014, Pages 885-897,

https://doi.org/10.1016/j.combustflame.2013.10.013.

**CombFlame2015/3755-Konnov**

Alexander A. Konnov, On the role of excited species in hydrogen combustion, Combustion and Flame, Volume 162, Issue 10, October 2015, Pages 3755-3772,

https://doi.org/10.1016/j.combustflame.2015.07.014.

**GRI-17-species-mech**

R. Sankaran, E.R. Hawkes, J.H. Chen, T.F. Lu, C.K. Law, "Structure of a spatially developing turbulent lean methane–air Bunsen flame," Proceedings of the Combustion Institute 31 (2007) 1291–1298.

**GRI-mech-3.0**

G. P. Smith, D. M. Golden, M. Frenklach, N. W. Moriarty, B. Eiteneer, M. Goldenberg, C. T. Bowman, R. K. Hanson, S. Song, W. C. Gardiner Jr, V. V. Lissianski, Z. Qin. GRI-Mech 3.0 [online] (1999).

http://www.me.berkeley.edu/gri_mech/

**Gasoline_2**

This is an update of the LLNL Gasoline Surrogate available at

https://www-pls.llnl.gov/?url=science_and_technology-chemistry-combustion-gasoline_surrogate

Received from the authors via email in October 2014.

**Gasoline_Surrogate**

Gasoline Surrogate

A detailed chemical kinetic mechanism for the simulation of gasoline surrogate mixtures has been assembled from existing LLNL mechanisms for n-heptane, iso-octane, toluene and C5-C6 olefins and validated using experimental data from shock tubes, stirred reactor, and rapid compression machines.

Mehl M., W.J. Pitz, C.K. Westbrook, H.J. Curran, "Kinetic modeling of gasoline surrogate components and mixtures under engine conditions", Proceedings of the Combustion Institute 33:193-200 (2011).

Downloaded from https://www-pls.llnl.gov/?url=science_and_technology-chemistry-combustion-gasoline_surrogate in September 2013

**H2**

"Comprehensive H2/O2 kinetic model for high-pressure combustion" Michael P. Burke, Marcos Chaos, Yiguang Ju, Frederick L. Dryer, and Stephen J. Klippenstein. International Journal of Chemical Kinetics, Volume 44, Issue 7, pages 444-474, July 2012.

https://doi.org/10.1002/kin.20603

Model last updated 2011-07-26.

**H2-3**

This is ”model 3” from a study on H2/O2 that was presented as a poster at the 36th International Symposium on Combustion. Seoul, South Korea. 31st July – 5th August, 2016: P. R. Westmoreland, S. Baskaran, M. P. Burke, M. Frenklach, C. D. Needham, J. Oreluk, U. Riedel, S. M. Sarathy, N. Slavinskaya, R. H. West. *Developing Combustion Mechanisms Dynamically as a Community.*

**IJCK2013/638-Metcalfe**

Metcalfe, Wayne K.; Burke, Sinéad M.; Ahmed, Syed S.; Curran, Henry J.; A Hierarchical and Comparative Kinetic Modeling Study of C1 − C2 Hydrocarbon and Oxygenated Fuels. *Int. J. Chem. Kinet.* 45(10):1097-4601

https://doi.org/10.1002/kin.20802

**MB-Dooley**

Methyl Butanoate. S. Dooley, H. J. Curran, J. M. Simmie. Combustion Chemistry Centre, National University of Ireland, Galway, University Road, Galway, Ireland.

Downloaded from http://c3.nuigalway.ie/methylbutanoate.html in May 2013. Reportedly from the following (although that contains no supplementary material.)

Dooley, S.; Curran, H. J.; Simmie, J. M. “Autoignition measurements and a validated kinetic model for the biodiesel surrogate, methyl butanoate.” Combust. Flame 2008, 153, 2–32

http://doi.org/10.1016/j.combustflame.2008.01.005

**MB-Farooq**

Farooq, A.; Ren, W.; Lam, K. Y.; Davidson, D. F.; Hanson, R. K.; Westbrook, C. K. ”Shock tube studies of methyl butanoate pyrolysis with relevance to biodiesel.” Combust. Flame 2012, 159, 3235-3241

http://doi.org/10.1016/j.combustflame.2012.05.013

**MB-Fisher**

Methyl Butanoate (and Methyl Formate) E. M. Fisher, W. J. Pitz, H. J. Curran, and C. K. Westbrook. Lawrence Livermore National Laboratory, Livermore, CA, UCRL-JC-137097.

Downloaded from https://www-pls.llnl.gov/?url=science_and_technology-chemistry-combustion-mbutanoate in May 2013. Reportedly from the following although that paper contains no supplementary material, and the files describe a few changes that were made since the symposium paper was published.

Fisher, E. M.; Pitz, W. J.; Curran, H. J.; Westbrook, C. K. “Detailed chemical kinetic mechanisms for combustion of oxygenated fuels.” Proc. Combust. Inst. 2000, 28, 1579–1586

http://doi.org/10.1016/S0082-0784(00)80555-X

**MatheuCH4**

Mechanism Generation with Integrated Pressure Dependence: A New Model for Methane Pyrolysis. David M. Matheu, Anthony M. Dean, Jeffrey M. Grenda, and William H. Green, J. Phys. Chem. A, 2003, 107 (41), pp 8552–8565

http://doi.org/10.1021/jp0345957

**Narayanaswamy**

Narayanaswamy, K., G. Blanquart, and H. Pitsch. ”A consistent chemical mechanism for oxidation of substituted aromatic species.” Combustion and Flame 157.10 (2010): 1879-1898.

https://doi.org/10.1016/j.combustflame.2010.07.009.

**PCI2013/225-Somers**

K.P. Somers, J.M. Simmie, F. Gillespie, U. Burke, J. Connolly, W.K. Metcalfe, F. Battin-Leclerc, P. Dirrenberger, O. Herbinet, P.-A. Glaude, H.J. Curran, A high temperature and atmospheric pressure experimental and detailed chemical kinetic modelling study of 2-methyl furan oxidation, Proceedings of the Combustion Institute, Volume 34, Issue 1, 2013, Pages 225-232,

https://doi.org/10.1016/j.proci.2012.06.113.

**PCI2013/259-Labbe**

Nicole J. Labbe, Vikram Seshadri, Tina Kasper, Nils Hansen, Patrick Oßwald, Phillip R. Westmoreland, Flame chemistry of tetrahydropyran as a model heteroatomic biofuel, Proceedings of the Combustion Institute, Volume 34, Issue 1, 2013, Pages 259-267,

https://doi.org/10.1016/j.proci.2012.07.027.

**PCI2013/269-Matsugi**

Akira Matsugi, Akira Miyoshi, Modeling of two- and three-ring aromatics formation in the pyrolysis of toluene, Proceedings of the Combustion Institute, Volume 34, Issue 1, 2013, Pages 269-277,

https://doi.org/10.1016/j.proci.2012.06.032.

**PCI2013/289-Dagaut**

P. Dagaut, A. Ristori, A. Frassoldati, T. Faravelli, G. Dayma, E. Ranzi, Experimental and semi-detailed kinetic modeling study of decalin oxidation and pyrolysis over a wide range of conditions, Proceedings of the Combustion Institute, Volume 34, Issue 1, 2013, Pages 289-296,

https://doi.org/10.1016/j.proci.2012.05.099.

**PCI2013/297-Herbinet**

Olivier Herbinet, Benoit Husson, Maude Ferrari, Pierre-Alexandre Glaude, Frédérique Battin-Leclerc, Low temperature oxidation of benzene and toluene in mixture with n-decane, Proceedings of the Combustion Institute, Volume 34, Issue 1, 2013, Pages 297-305,

https://doi.org/10.1016/j.proci.2012.06.005.

**PCI2013/325-Husson**

Benoit Husson, Maude Ferrari, Olivier Herbinet, Syed S. Ahmed, Pierre-Alexandre Glaude, Frédérique Battin-Leclerc, New experimental evidence and modeling study of the ethylbenzene oxidation, Proceedings of the Combustion Institute, Volume 34, Issue 1, 2013, Pages 325-333,

https://doi.org/10.1016/j.proci.2012.06.002.

**PCI2013/335-Wang**

Weijing Wang, Zhenhua Li, Matthew A. Oehlschlaeger, Darren Healy, Henry J. Curran, S. Mani Sarathy, Marco Mehl, William J. Pitz, Charles K. Westbrook, An experimental and modeling study of the autoignition of 3-methylheptane, Proceedings of the Combustion Institute, Volume 34, Issue 1, 2013, Pages 335-343,

https://doi.org/10.1016/j.proci.2012.06.001.

**PCI2013/353-Malewicki**

Tomasz Malewicki, Andrea Comandini, Kenneth Brezinsky, Experimental and modeling study on the pyrolysis and oxidation of iso-octane, Proceedings of the Combustion Institute, Volume 34, Issue 1, 2013, Pages 353-360,

https://doi.org/10.1016/j.proci.2012.06.137.

**PCI2013/361-Malewicki**

Tomasz Malewicki, Kenneth Brezinsky, Experimental and modeling study on the pyrolysis and oxidation of n-decane and n-dodecane, Proceedings of the Combustion Institute, Volume 34, Issue 1, 2013, Pages 361-368,

https://doi.org/10.1016/j.proci.2012.06.156.

**PCI2013/401-Liu**

W. Liu, R. Sivaramakrishnan, Michael J. Davis, S. Som, D.E. Longman, T.F. Lu, Development of a reduced biodiesel surrogate model for compression ignition engine modeling, Proceedings of the Combustion Institute, Volume 34, Issue 1, 2013, Pages 401-409,

https://doi.org/10.1016/j.proci.2012.05.090.

**PCI2013/411-Darcy**

D. Darcy, M. Mehl, J.M. Simmie, J. Würmel, W.K. Metcalfe, C.K. Westbrook, W.J. Pitz, H.J. Curran, An experimental and modeling study of the shock tube ignition of a mixture of n-heptane and n-propylbenzene

as a surrogate for a large alkyl benzene, Proceedings of the Combustion Institute, Volume 34, Issue 1, 2013, Pages 411-418,

https://doi.org/10.1016/j.proci.2012.06.131.

**PCI2013/527-Sheen**
David A. Sheen, Claudette M. Rosado-Reyes, Wing Tsang, Kinetics of H atom attack on unsaturated hydrocarbons using spectral uncertainty propagation and minimization techniques, Proceedings of the Combustion Institute, Volume 34, Issue 1, 2013, Pages 527-536,

https://doi.org/10.1016/j.proci.2012.06.062.

**PCI2013/599-Veloo**
P.S. Veloo, P. Dagaut, C. Togbe, G. Dayma, S.M. Sarathy, C.K. Westbrook, F.N. Egolfopoulos, Jet-stirred reactor and flame studies of propanal oxidation, Proceedings of the Combustion Institute, Volume 34, Issue 1, 2013, Pages 599-606,

https://doi.org/10.1016/j.proci.2012.06.138.

**PCI2015/0153-Marshall**
Paul Marshall, Peter Glarborg, Ab initio and kinetic modeling studies of formic acid oxidation, Proceedings of the Combustion Institute, Volume 35, Issue 1, 2015, Pages 153-160,

https://doi.org/10.1016/j.proci.2014.05.091.

**PCI2015/0325-Nawdiyal**
A. Nawdiyal, N. Hansen, T. Zeuch, L. Seidel, F. Mauß, Experimental and modelling study of speciation and benzene formation pathways in premixed 1-hexene flames, Proceedings of the Combustion Institute, Volume 35, Issue 1, 2015, Pages 325-332,

https://doi.org/10.1016/j.proci.2014.06.047.

**PCI2015/0409-Zhang**
Xiaoyuan Zhang, Bin Yang, Wenhao Yuan, Zhanjun Cheng, Lidong Zhang, Yuyang Li, Fei Qi, Pyrolysis of 2-methyl-1-butanol at low and atmospheric pressures: Mass spectrometry and modeling studies, Proceedings of the Combustion Institute, Volume 35, Issue 1, 2015, Pages 409-417,

https://doi.org/10.1016/j.proci.2014.06.080.

**PCI2017/012-Felsmann**
Daniel Felsmann, Hao Zhao, Qiang Wang, Isabelle Graf, Ting Tan, Xueliang Yang, Emily A. Carter, Yiguang Ju, Katharina Kohse-Höinghaus, Contributions to improving small ester combustion chemistry: Theory, model and experiments, Proceedings of the Combustion Institute, Available online 11 June 2016,

https://doi.org/10.1016/j.proci.2016.05.012.

**PCI2017/022-Thion**
Sébastien Thion, Pascal Diévart, Pierre Van Cauwenberghe, Guillaume Dayma, Zeynep Serinyel, Philippe Dagaut, An experimental study in a jet-stirred reactor and a comprehensive kinetic mechanism for the oxidation of methyl ethyl ketone, Proceedings of the Combustion Institute, Available online 11 June 2016,

https://doi.org/10.1016/j.proci.2016.05.022.

**PCI2017/024-Bohon**
Myles D. Bohon, Thibault F. Guiberti, S. Mani Sarathy, William L. Roberts, Variations in non-thermal NO formation pathways in alcohol flames, Proceedings of the Combustion Institute, Available online 4 July 2016,

https://doi.org/10.1016/j.proci.2016.05.024.

**PCI2017/025-Sudholt**
Alena Sudholt, Rupali Tripathi, Daniel Mayer, Pierre-Alexandre Glaude, Frédérique Battin-Leclerc, Heinz Pitsch, The oxidation of the novel lignocellulosic biofuel $\gamma$-valerolactone in a low pressure flame, Proceedings of the Combustion Institute, Available online 14 June 2016,

https://doi.org/10.1016/j.proci.2016.05.025.

**PCI2017/032-Cheng**
Zhanjun Cheng, Qi Niu, Zhandong Wang, Hanfeng Jin, Guanyi Chen, Mingfa Yao, Lixia Wei, Experimental and kinetic modeling studies of low-pressure premixed laminar 2-methylfuran flames, Proceedings of the Combustion Institute, Available online 19 July 2016,

https://doi.org/10.1016/j.proci.2016.07.032.

**PCI2017/036-Rashidi**
Mariam J. Al Rashidi, Sébastien Thion, Casimir Togbé, Guillaume Dayma, Marco Mehl, Philippe Dagaut, William J. Pitz, Judit Zádor, S. Mani Sarathy, Elucidating reactivity regimes in cyclopentane oxidation: Jet stirred reactor experiments, computational chemistry, and kinetic modeling, Proceedings of the Combustion Institute, Available online 22 June 2016,

https://doi.org/10.1016/j.proci.2016.05.036.

**PCI2017/037-Sakai**
Yasuyuki Sakai, Jürgen Herzler, Marc Werler, Christof Schulz, Mustapha Fikri, A quantum chemical and kinetics modeling study on the autoignition mechanism of diethyl ether, Proceedings of the Combustion Institute, Available online 16 June 2016,

https://doi.org/10.1016/j.proci.2016.06.037.

**PCI2017/038-Labbe-Zhao(30Torr-10Atm)**
Nicole J. Labbe, Raghu Sivaramakrishnan, C. Franklin Goldsmith, Yuri Georgievskii, James A. Miller, Stephen J. Klippenstein, Ramifications of including non-equilibrium effects for HCO in flame chemistry, Proceedings of the Combustion Institute, Available online 24 June 2016,

https://doi.org/10.1016/j.proci.2016.06.038.

**PCI2017/047-Rodriguez**
Anne Rodriguez, Olivier Herbinet, Frédérique Battin-Leclerc, A study of the low-temperature oxidation of a long chain aldehyde: n-hexanal, Proceedings of the Combustion Institute, Available online 16 June 2016,

https://doi.org/10.1016/j.proci.2016.05.047.

**PCI2017/051-Pelucchi**
Matteo Pelucchi, Eliseo Ranzi, Alessio Frassoldati, Tiziano Faravelli, Alkyl radicals rule the low temperature oxidation of long chain aldehydes, Proceedings of the Combustion Institute, Available online 16 June 2016,

https://doi.org/10.1016/j.proci.2016.05.051.

**PCI2017/052-Li**
Yang Li, Chong-Wen Zhou, Kieran P. Somers, Kuiwen Zhang, Henry J. Curran, The oxidation of 2-butene: A high pressure ignition delay, kinetic modeling study and reactivity comparison with isobutene and 1-butene, Proceedings of the Combustion Institute, Available online 16 June 2016,

https://doi.org/10.1016/j.proci.2016.05.052.

**PCI2017/052-Stagni**
A. Stagni, L. Esclapez, P. Govindaraju, A. Cuoci, T. Faravelli, M. Ihme, The role of preferential evaporation on the ignition of multicomponent fuels in a homogeneous spray/air mixture, Proceedings of the Combustion Institute, Available online 21 June 2016,

https://doi.org/10.1016/j.proci.2016.06.052.

**PCI2017/058-Sun**
Wenyu Sun, Guoqing Wang, Shuang Li, Ruzheng Zhang, Bin Yang, Jiuzhong Yang, Yuyang Li, Charles K. Westbrook, Chung K. Law, Speciation and the laminar burning velocities of poly(oxymethylene) dimethyl ether 3 (POMDME3) flames: An experimental and modeling study, Proceedings of the Combustion Institute, Available online 16 June 2016,

https://doi.org/10.1016/j.proci.2016.05.058.

**PCI2017/082-Hemken**
Christian Hemken, Ultan Burke, Isabelle Graf, Lena Ruwe, Sungwoo Park, S. Mani Sarathy, K. Alexander Heufer, Katharina Kohse-Höinghaus, A laminar flame investigation of 2-butanone, and the combustion-related intermediates formed through its oxidation, Proceedings of the Combustion Institute, Available online 22 June 2016,

https://doi.org/10.1016/j.proci.2016.06.082.

**PCI2017/087-Tran**

Luc-Sy Tran, Julia Pieper, Hans-Heinrich Carstensen, Hao Zhao, Isabelle Graf, Yiguang Ju, Fei Qi, Katharina Kohse-Höinghaus, Experimental and kinetic modeling study of diethyl ether flames, Proceedings of the Combustion Institute, Available online 24 June 2016,

https://doi.org/10.1016/j.proci.2016.06.087.

**PCI2017/111-Jin**

Hanfeng Jin, Guoqing Wang, Yizun Wang, Xiaoyuan Zhang, Yuyang Li, Zhongyue Zhou, Jiuzhong Yang, Fei Qi, Experimental and kinetic modeling study of laminar coflow diffusion methane flames doped with isobutanol, Proceedings of the Combustion Institute, Available online 25 June 2016,

https://doi.org/10.1016/j.proci.2016.06.111.

**PCI2017/145-Sun**

Wenyu Sun, Bin Yang, Nils Hansen, Kai Moshammer, The influence of dimethoxy methane (DMM)/dimethyl carbonate (DMC) addition on a premixed ethane/oxygen/argon flame, Proceedings of the Combustion Institute, Available online 4 July 2016,

https://doi.org/10.1016/j.proci.2016.06.145.

**Reduced-DRG-GRI-mech**

GRI-Mech 3.0 reduced using Directed Relation Graph method.

**Shamel-Propane**

A mechanism for propane made by Shamel Merchant (at MIT) using RMG-Java.

**USC_Mech_ii**

Hai Wang, Xiaoqing You, Ameya V. Joshi, Scott G. Davis, Alexander Laskin, Fokion Egolfopoulos & Chung K. Law, USC Mech Version II. High-Temperature Combustion Reaction Model of H2/CO/C1-C4 Compounds.

http://ignis.usc.edu/USC_Mech_II.htm, May 2007.

Downloaded in August 2013 from
http://ignis.usc.edu/Mechanisms/USC-Mech%20II/USC_Mech%20II.htm

**n-Heptane**

n-Heptane, Detailed Mechanism, Version 3.1

This mechanism represents an updated release of the previous version available on the website (Version 3.0). The mechanism is based on the previously developed and very successful mechanism of Curran et al. 1998 (Combust. Flame 114:149-177). Version 3.1 fixes some bugs found in Version 3.0.

References for Mechanism

Mehl M., W.J. Pitz, C.K. Westbrook, H.J. Curran, ”Kinetic Modeling of Gasoline Surrogate Components and Mixtures Under Engine Conditions”, Proceedings of the Combustion Institute 33:193-200 (2011).

M. Mehl, W. J. Pitz, M. Sjöberg and J. E. Dec, ”Detailed kinetic modeling of low-temperature heat release for PRF fuels in an HCCI engine,” SAE 2009 International Powertrains, Fuels and Lubricants Meeting, SAE Paper No. 2009-01-1806, Florence, Italy, 2009. Available at www.sae.org.

Downloaded in September 2013 from
https://www-pls.llnl.gov/?url=science_and_technology-chemistry-combustion-n_heptane_version_3
